# Supplementary material for: Learning to Represent Surroundings, Anticipate Motion and Take Informed Actions in Unstructured Environments
Source: arXiv:2407.10383 source file (2024-07-15)
Supplement: Supplementary file 1 [file appendix.tex]

Appendix goes here.
